# Supplementary material for: The Limitations of Stylometry for Detecting Machine-Generated Fake News
Source: arXiv:1908.09805 source file (2020-02-20)
Supplement: Supplementary file 1 [file appendix.tex]

\section{Veracity-based QA Dataset}

We simulate a scenario where real text is produced by an auto-completion tool and verifies for correctness, whereas an attacker uses the same tool, but verifies \emph{in}correctness. 
To this end, we use the newsQA dataset~\citep{trischler-etal-2017-newsqa} that contains CNN articles and questions about them. Following the setting of \citet{radford2019language}, we append a template to the end of the article in order to apply the generator as a zero-shot question-answering model. We use the format below to append the question:

% \begin{tabular}{ll}
%  \verb|We attempt to answer: <question>|  & \textit{what is ..} \\
%   \verb|Answer: |   & a asfd
% \end{tabular}
\begin{verbatim}
We attempt to answer: <question>
Answer: \end{verbatim} 
Then, the first sentence produced by Grover's generator is used as a potential answer. This template was chosen by examining common formats of questions in news articles and was found to produce reasonable results by Grover's generator.\footnote{Evaluating against the dataset's ground-truth answers, Grover achieved token-level overlap F1 score of 0.19 on newsQA's test set and of 0.25 on our filtered evaluation set.} For example, for an article about a man caught with a gun, the following answer was generated based on the article and the appended question:\\

\noindent \verb|We attempt to answer: Where was the suspect stopped?|\\
\verb|Answer: |\textit{2 blocks from the U.S. Capitol.}\\
For more examples, see \figref{fig:examples}.
%Following one of the use cases of \citet{radford2019language}, we append . To this end, we append the following text to the end of the article: 
%\begin{verbatim}\nWe attempt to answer:<question>.\nAnswer:\end{verbatim} 
%were \texttt{<question>} is replaced with a question about the article. We modified Grover to begin its generation from the end of this added text and use the first generated sentence as an answer. 

We generated 1000 such answers and manually filtered nonsensical statements, i.e.\ that did not look like a suitable (true or false) answer to the given question. This resulted in about 700 answers labeled as true or false according to the correctness of their content. Finally, the cases were split to 30\% for evaluation and the rest for fine-tuning. 
Since the gold answer from the newsQA dataset is a span from the article, after appending the human/machine answers, we remove the article's sentence with the highest word count tf-idf similarity with the question and answer (concatenated). This simulates a scenario where the writer provides additional information about the article's topic, and it prevents the discriminator from simply matching exact phrases.
The dataset consists of:

\noindent \underline{Real text:} CNN articles with an appended question and a generated answer that was marked as true.\\
\underline{Fake text:}
CNN articles with an appended question and a generated answer that was marked as false.

%we used 30\% of them for evaluation and the rest for fine-tuning.
%\begin{verbatim}\nWe attempt to answer:<question>.\nAnswer:\end{verbatim} 

Only answers that contained entirely true facts were labeled as real. Answers containing at least one false statement were labeled fake. About 45\% of Grover's answers were real (post the nonsensical filtering).

%%%%%%%%%%%%%%%%%%%%%%%%%%%%%%%%%%%%%%%%%%%%%%%%%%%%%%%%%%%%%%%%%%%%%%%%%%%%%

\section{Zero-shot attacks}

\subsection{Full Text attack} \label{app:fulltext}

\begin{figure}[t]
  \centering
  \subfloat[temperature 1]{\includegraphics[width=0.7\textwidth]{figures/temp1_conf.png}\label{fig:f1}}
%   \hfill
\\ \vspace{-5mm}
  \subfloat[Top-K 40]{\includegraphics[width=0.7\textwidth]{figures/k40_conf.png}\label{fig:f2}}
  \caption{Confusion matrices for Grover Fake text detection on the unconditional generations of the GPT2-XL model with temperature 1 (a) and with Top-K 40 sampling (b).}
\end{figure}

\begin{figure}[t]
  \centering
  \subfloat[Temperature 1]{\includegraphics[width=0.5\textwidth]{figures/temp1_roc.png}}
  \hfill
  \subfloat[Top-K 40]{\includegraphics[width=0.5\textwidth]{figures/k40_roc.png}}
  \caption{ROC curve for Grover Fake text detection on the unconditional generations of the GPT2-XL model with temperature 1 (left) and with Top-K 40 sampling (right).} \label{fig:roc}
\end{figure}

\begin{figure}[t]
  \centering
  \subfloat[Input=250 tokens]{\includegraphics[width=0.7\textwidth]{figures/conditional_250.png}}
  \\
  \subfloat[Input=500 tokens]{\includegraphics[width=0.7\textwidth]{figures/conditional_500.png}}
\caption{Percent of cases that Grover predicted as real by the fraction of added machine-generated tokens from the input human-written tokens.}
\label{fig:grov_pred_hum}
\end{figure}

\tal{TODO- write this. zero shot for full article and for extensions (500 and 250)}

For each sentence that added, we run Grover's discriminator and check if it predicts the article as human written. For evaluation, we count the number of tokens in the human-written text and report the prediction of Grover by the fraction of the machine-generated tokens from the original text (1.0 means that the extended article is double the size of the original).

Since obviously the source of each sentence is hidden, Grover's discriminator is applied over the full article to predict if it's fake or real. We note that an attempt to classify each sentence separately is not supported by Grover (their web interface doesn't accept it and asks for a full article).

The ROC curve (see \appref{app:fulltext}) shows that potentially better trade-off points are attainable.
