# Supplementary material for: The Limitations of Stylometry for Detecting Machine-Generated Fake News
Source: arXiv:1908.09805 source file (2020-02-20)
Supplement: Supplementary file 2 [file appendix-training.tex]

\section{Fine-tuning Technical Details}

For the fine-tuning defense, we fine-tuned a Grover-Mega model to distinguish between the two classes. For this setting, we used about 1000 examples where half were in the ``fake'' class. Fine-tuning was done for 10 epochs with a batch size of 16 on 8 TPU v3 cores. Comparable results can be achieved by fine-tuning on CPUs for 3 epochs with a batch size of 8 on a 40-core machine with 192 Gb ram. This setup takes 18 hours for a training set of 1000 samples.
